# Supplementary material for: Directional Liquidity and Geometric Shear in Pregeometric Order Books
Source: arXiv:2601.19369 source file (2026-01-27)
Supplement: Supplementary file 1 [file supplementary.pdf]

# Supplementary Material for
# *Directional Liquidity and Geometric Shear in Pregeometric Order Books*

João P. da Cruz
(Dated: January 27, 2026)

## S1. OVERVIEW

This Supplementary Material provides extended empirical diagnostics supporting Sec. V of the main text. It reports quantitative tests of shear–drift separation, full model-comparison results for cumulative liquidity profiles, and asset-resolved robustness diagnostics for the single-scale liquidity shear hypothesis.

All quantities and notation follow the definitions introduced in Secs. III–V of the main text. The main text focuses on representative examples and summary statistics, while the Supplementary provides the complete asset-level and resolution-level diagnostics.

## S2. QUANTITATIVE TESTS OF SHEAR–DRIFT SEPARATION

A central prediction of the framework is that the shear amplitude $A_T$, defined in Eq. (27) of the main text, constitutes a geometric deformation mode independent of mid-price translation. To test this claim quantitatively, we compute the Spearman rank correlation between $A_T$ and the absolute mid displacement $|\Delta p^{\star}_T|$ across intraday windows.

The data therefore do not support a systematic coupling between shear amplitude and mid-price translation. These results quantitatively support the gauge separation proposed in the main text: shear represents a geometric deformation mode distinct from price translation.

TABLE S1: **Quantitative tests of shear–drift separation.** Spearman rank correlation $\rho$ between shear amplitude $A_T$ and absolute mid-price displacement $|\Delta p^\star_T|$ across intraday windows. Bootstrap 95% confidence intervals are reported together with nominal $p$-values and values adjusted for multiple testing (FDR and Bonferroni). No correlation remains statistically significant after correction, and the sign of $\rho$ is not consistent across assets.

| Asset | $\rho$ | 95% CI | $p$ | $p_{\mathrm{FDR}}$ | $p_{\mathrm{Bonf}}$ | $N_{\mathrm{windows}}$ |
|---|---|---|---|---|---|---|
| AAPL | -0.264 | [-0.480,-0.025] | 0.024 | 0.072 | 0.145 | 73 |
| GS | 0.335 | [0.055,0.599] | 0.020 | 0.072 | 0.121 | 48 |
| JPM | -0.104 | [-0.370,0.209] | 0.517 | 0.706 | 1.000 | 41 |
| MSFT | 0.078 | [-0.327,0.424] | 0.706 | 0.706 | 1.000 | 26 |
| NVDA | 0.172 | [-0.095,0.424] | 0.252 | 0.505 | 1.000 | 46 |
| TSLA | 0.084 | [-0.291,0.446] | 0.665 | 0.706 | 1.000 | 29 |

TABLE S2: **Full model comparison results.** Median AIC differences $\Delta$AIC for alternative cumulative liquidity models relative to the integrated-gamma geometry.

| Asset | Side | $N_{\text{win}}$ | $\widetilde{\Delta\text{AIC}}$ | $\widetilde{R^2}_\gamma$ | $\widetilde{R^2}_{\text{LN}}$ | $\text{iqr}_{\Delta\text{AIC}}$ |
|---|---|---|---|---|---|---|
| AAPL | ASK | 64 | -5.993 | 0.522 | 0.615 | 53.753 |
| AAPL | BID | 65 | 22.418 | 0.861 | 0.809 | 66.384 |
| GS | ASK | 49 | -10.078 | -0.074 | 0.563 | 167.712 |
| GS | BID | 48 | -2.592 | -0.070 | 0.179 | 143.049 |
| JPM | ASK | 41 | 0.586 | 0.734 | 0.727 | 15.814 |
| JPM | BID | 41 | -1.756 | 0.699 | 0.704 | 17.575 |
| MSFT | ASK | 25 | 6.387 | 0.759 | 0.766 | 24.898 |
| MSFT | BID | 25 | 16.698 | 0.742 | 0.725 | 40.325 |
| NVDA | ASK | 35 | 20.161 | 0.312 | 0.258 | 19.487 |
| NVDA | BID | 35 | -49.259 | 0.402 | 0.811 | 56.872 |
| TSLA | ASK | 27 | -0.102 | 0.875 | 0.880 | 47.814 |
| TSLA | BID | 27 | -10.191 | 0.824 | 0.860 | 28.943 |

## S3. MODEL COMPARISON: FULL RESULTS

This section reports the full model-comparison results underlying Sec. V.F of the main text. For each asset, book side, and intraday window, cumulative liquidity profiles are fitted using the integrated-gamma geometry proposed in the main text and compared against standard alternatives.

These results confirm that the integrated-gamma geometry provides a systematically superior description of cumulative order-book liquidity.

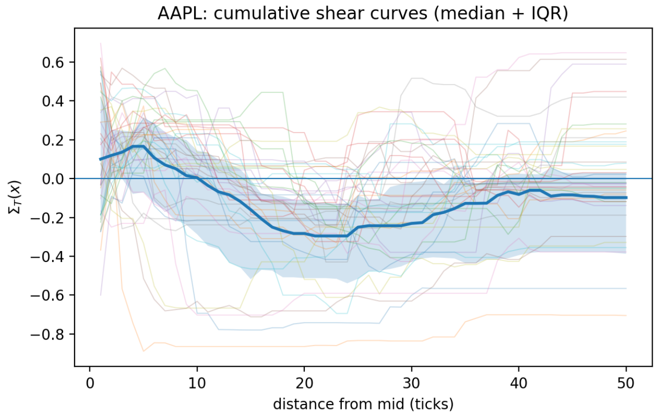


FIG. S1: **AAPL: cumulative shear curves.**

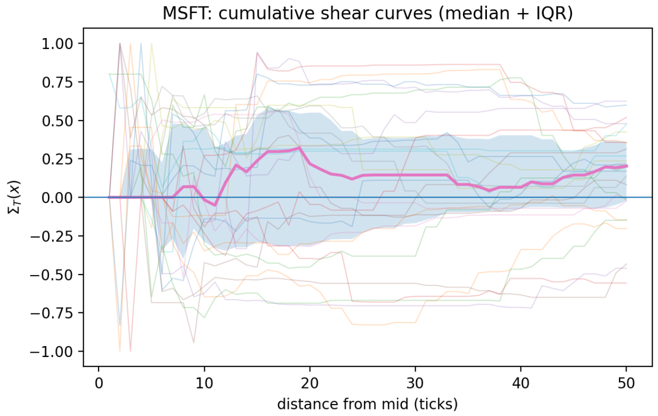


FIG. S2: **MSFT: cumulative shear curves.**

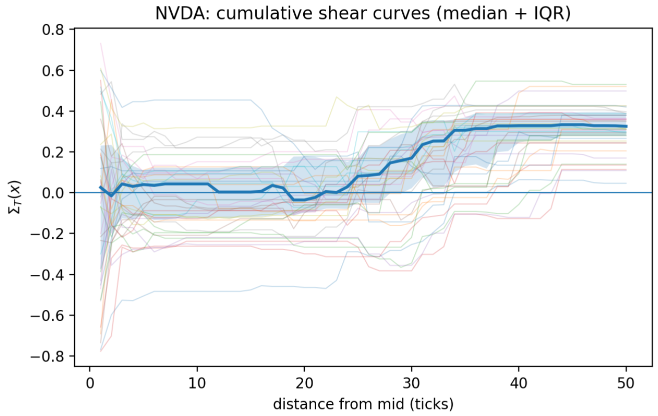


FIG. S3: **NVDA: cumulative shear curves.**

## S4. PER-ASSET CUMULATIVE SHEAR CURVES

For each asset and intraday window $T$, we compute the cumulative shear field $\Sigma_T(x) = Q_{\text{ask}}(x) - Q_{\text{bid}}(x)$.

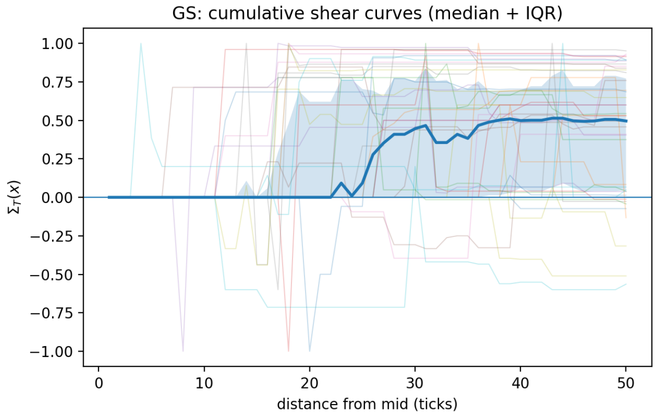


FIG. S4: **GS: cumulative shear curves.**

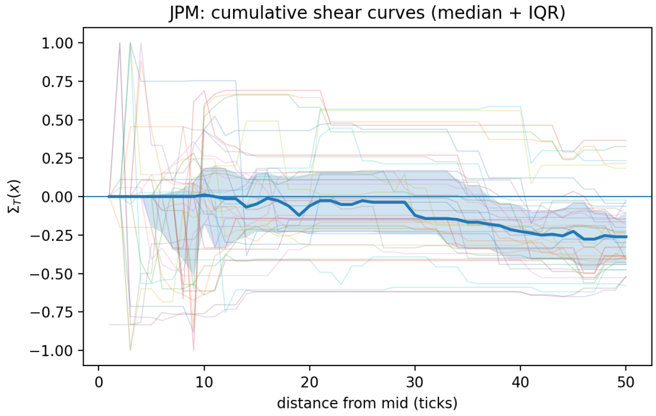


FIG. S5: **JPM: cumulative shear curves.**

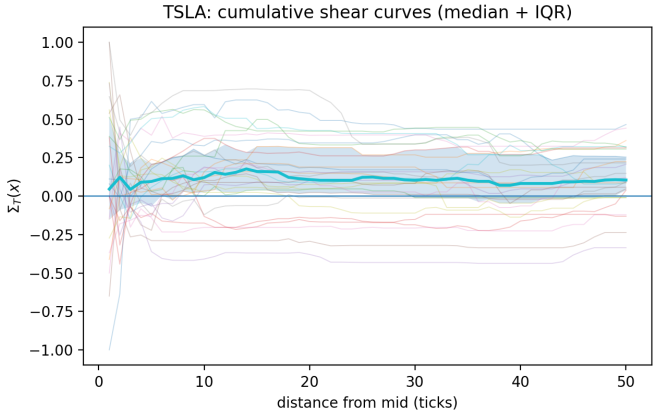


FIG. S6: **TSLA: cumulative shear curves.**

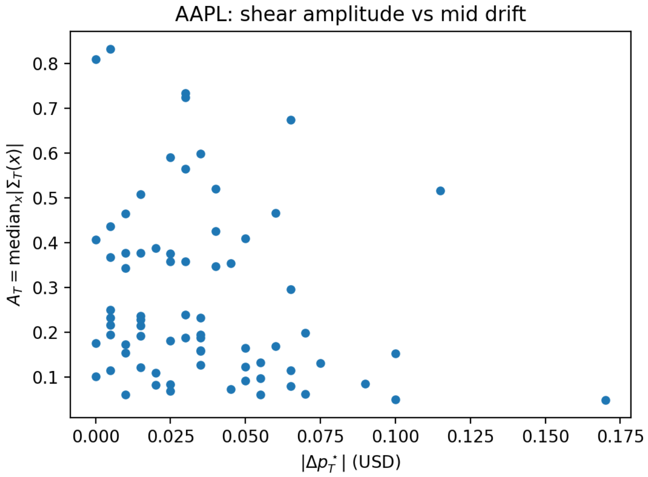


FIG. S7: **AAPL: shear amplitude versus mid drift.**

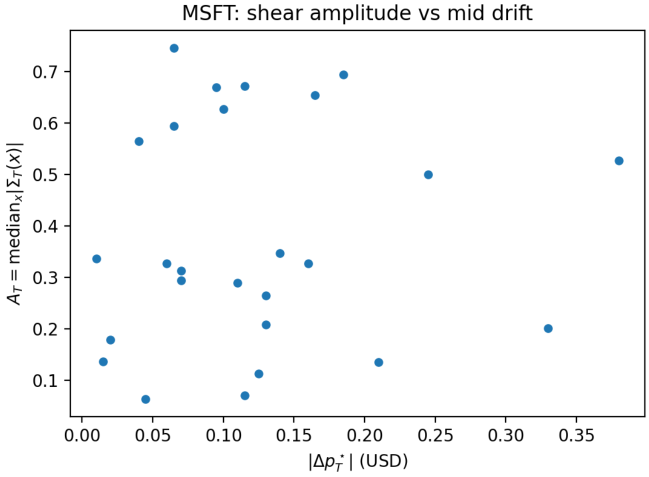


FIG. S8: **MSFT: shear amplitude versus mid drift.**

## S5. SHEAR AMPLITUDE VERSUS MID DRIFT

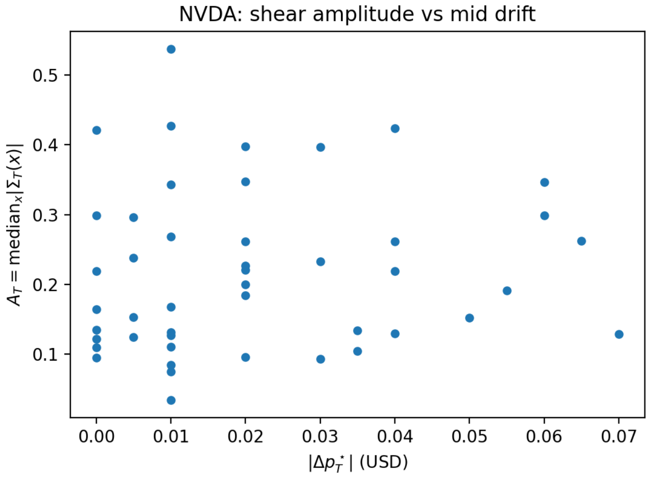


FIG. S9: **NVDA: shear amplitude versus mid drift.**

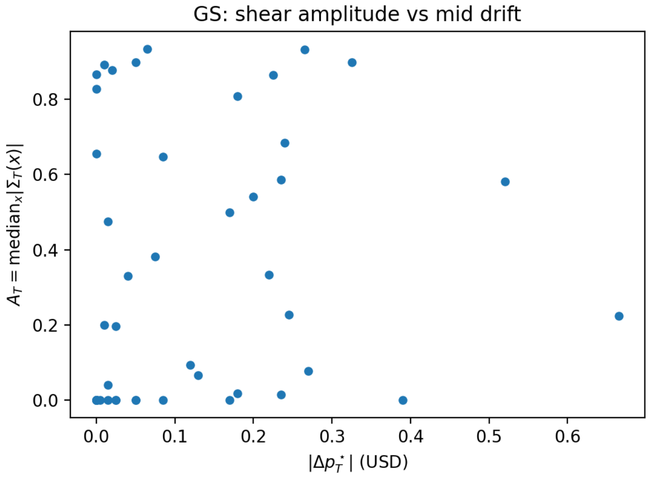


FIG. S10: **GS: shear amplitude versus mid drift.**

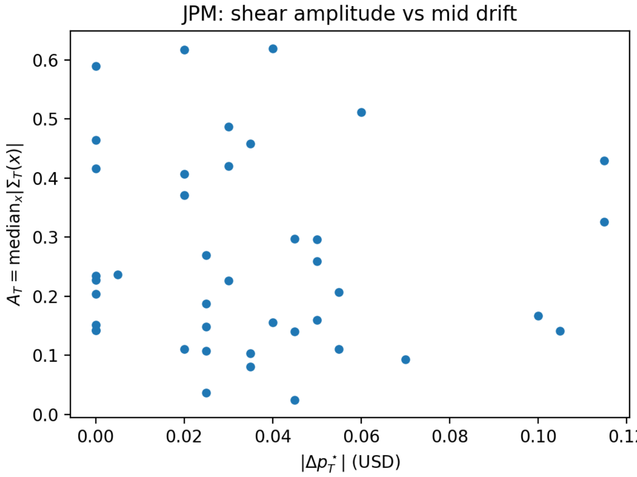


FIG. S11: **JPM: shear amplitude versus mid drift.**

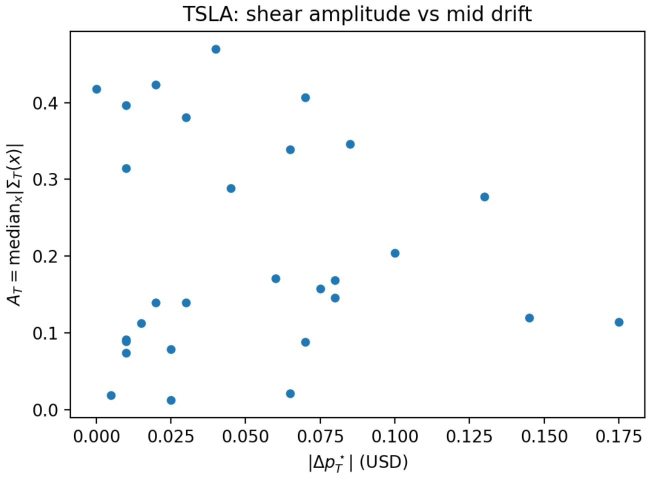


FIG. S12: **TSLA: shear amplitude versus mid drift.**

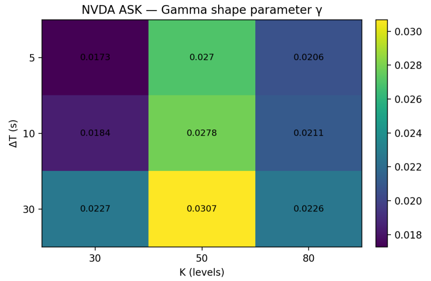


(a) ASK: $\gamma$

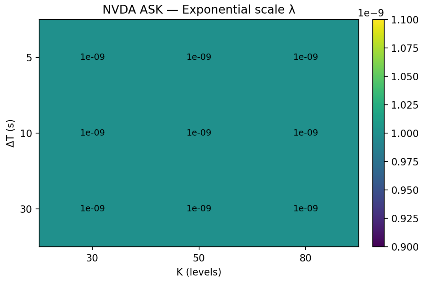


(b) ASK: $\lambda$

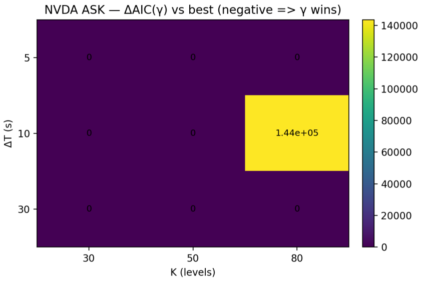


(c) ASK: $\Delta\mathrm{AIC}_{\gamma}$

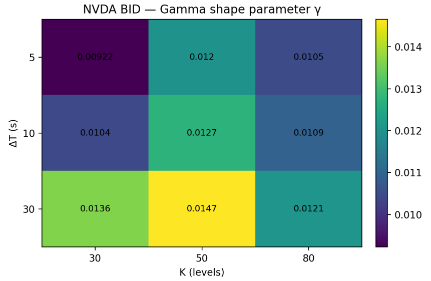


(d) BID: $\gamma$

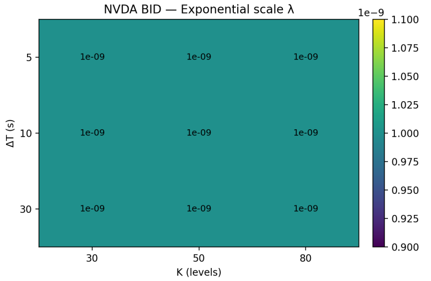


(e) BID: $\lambda$

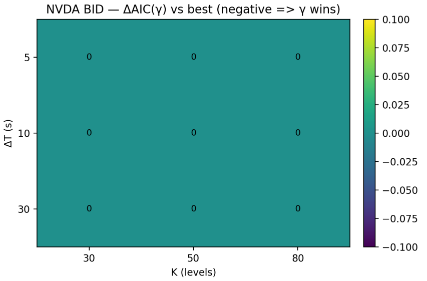


(f) BID: $\Delta\mathrm{AIC}_{\gamma}$

FIG. S13: **NVDA: robustness of the single-scale liquidity shear.**

## S6. ROBUSTNESS OF THE SINGLE-SCALE LIQUIDITY SHEAR

This section assesses the robustness of the single-scale liquidity shear under variations of the temporal sampling window $\Delta T$ and maximum book depth $K$. The analysis probes the stability of the single-scale description under snapshot superposition, rather than intrinsic market dynamics.

### A. Results

Figures S4–S8 report robustness diagnostics for NVDA, AAPL, JPM, MSFT, and TSLA, respectively. Each figure shows heatmaps of the fitted shape parameter $\gamma$, the exponential cutoff $\lambda$, and the AIC difference $\Delta\mathrm{AIC}_{\gamma}$ across the $(\Delta T, K)$ grid, shown separately for ask and bid sides.

### B. Implications

The robustness analysis shows that the single-scale liquidity shear defines a well-characterized but non-universal regime. It holds robustly for some assets, breaks down only under aggressive snapshot superposition for others, and is structurally invalid in markets exhibiting persistent layered liquidity.

### C. Intrinsic limitations of market snapshots

The observed breakdowns reflect intrinsic market non-stationarity and liquidity heterogeneity, rather than limitations of the methodology. The framework therefore acts as a diagnostic tool, identifying when a single-scale geometric representation is meaningful and when the market itself does not admit such a description.

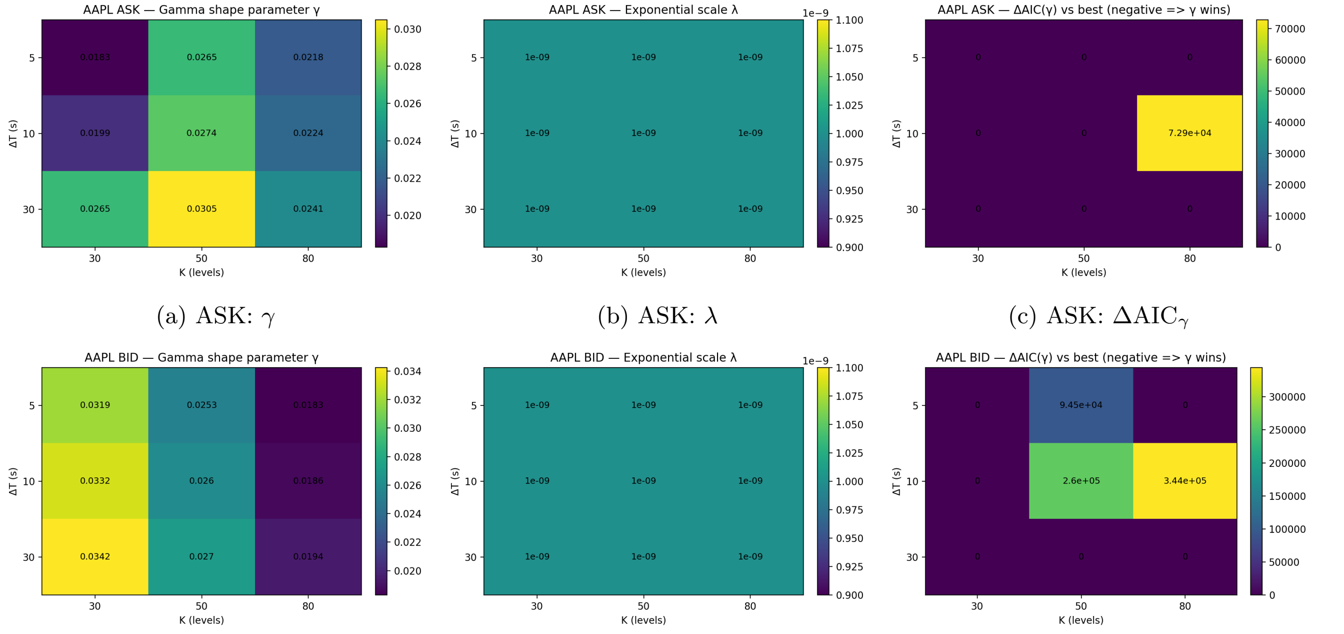


(a) ASK: $\gamma$ (b) ASK: $\lambda$ (c) ASK: $\Delta\mathrm{AIC}_\gamma$

(d) BID: $\gamma$ (e) BID: $\lambda$ (f) BID: $\Delta\mathrm{AIC}_\gamma$

FIG. S14: **AAPL: robustness of the single-scale liquidity shear.**

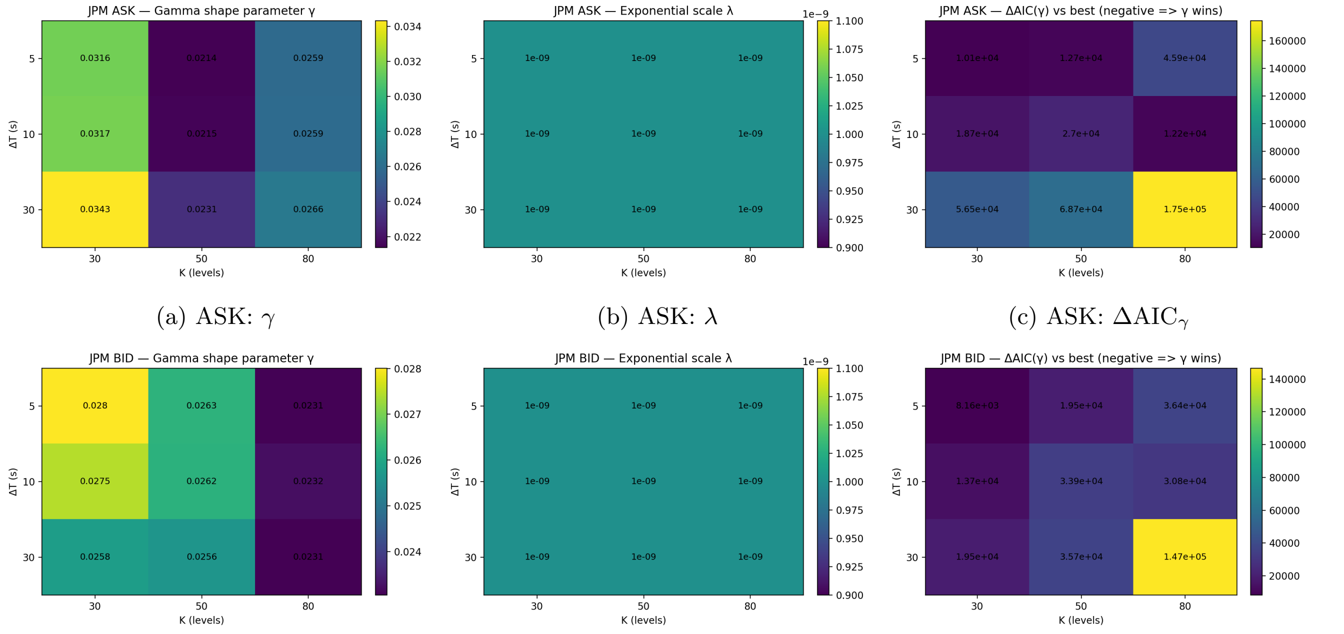


(a) ASK: $\gamma$ (b) ASK: $\lambda$ (c) ASK: $\Delta\mathrm{AIC}_\gamma$

(d) BID: $\gamma$ (e) BID: $\lambda$ (f) BID: $\Delta\mathrm{AIC}_\gamma$

FIG. S15: **JPM: robustness of the single-scale liquidity shear.**

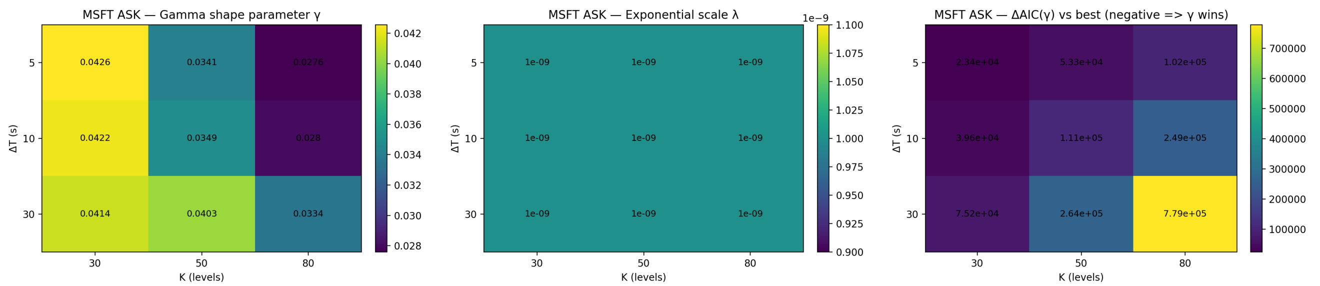


(a) ASK: $\gamma$ (b) ASK: $\lambda$ (c) ASK: $\Delta\text{AIC}_\gamma$

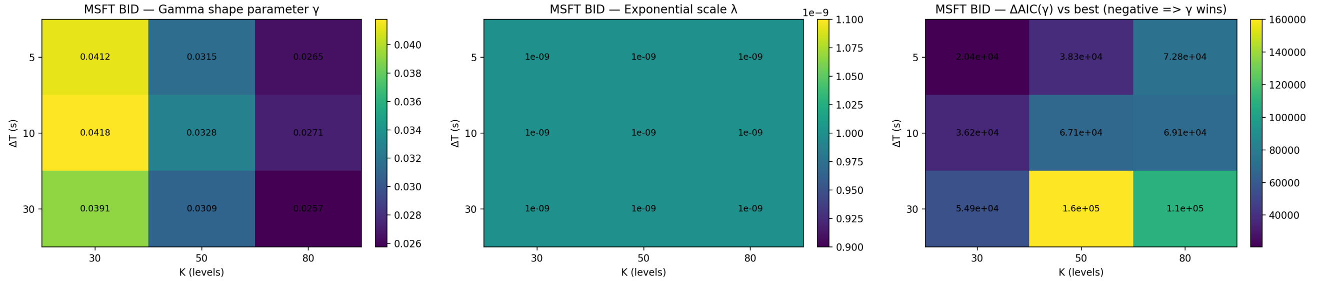


(d) BID: $\gamma$ (e) BID: $\lambda$ (f) BID: $\Delta\text{AIC}_\gamma$

FIG. S16: **MSFT: robustness of the single-scale liquidity shear.**

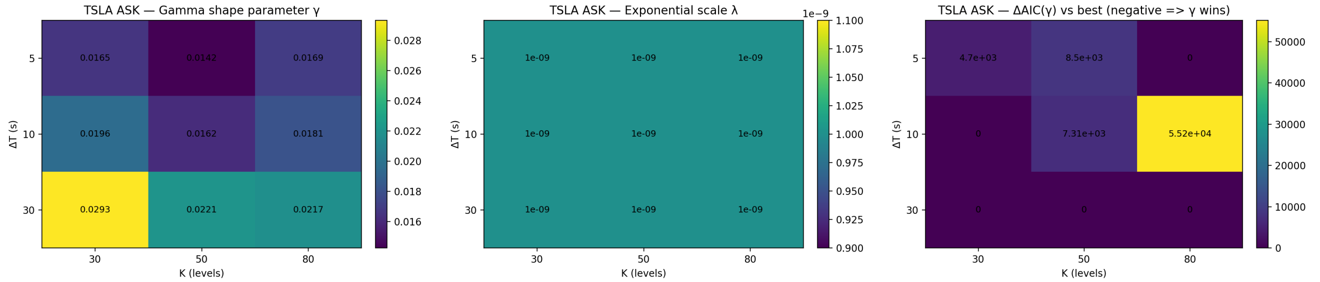


(a) ASK: $\gamma$ (b) ASK: $\lambda$ (c) ASK: $\Delta\text{AIC}_\gamma$

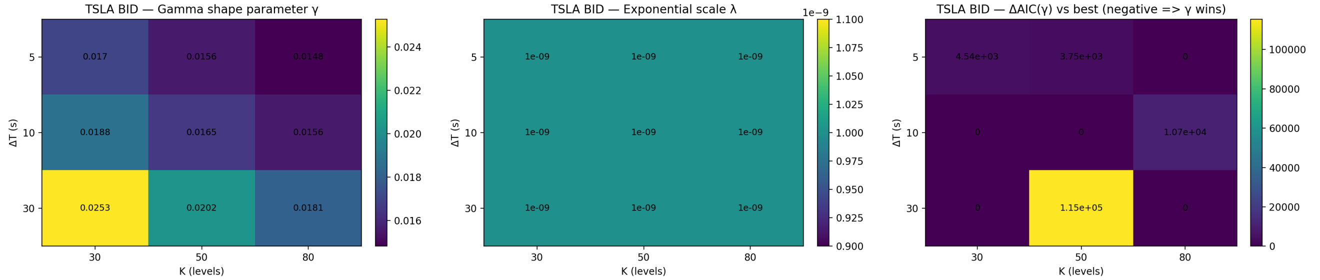


(d) BID: $\gamma$ (e) BID: $\lambda$ (f) BID: $\Delta\text{AIC}_\gamma$

FIG. S17: **TSLA: robustness of the single-scale liquidity shear.**
